# Supplementary material for: Reasoning with Probabilities: Relating Weighted Model Counting and Probabilistic Model Checking
Source: arXiv:2608.22632 source file (2026-08-23)
Supplement: Supplementary file 1 [file appendix-proof.tex]

\begin{proof}[Proof of Proposition \ref{prop-mc-to-ac}] Let $\M$ be an acyclic path-compatible pMC and $\mathcal{C}_{\M}$ be its AC obtained from Def. \ref{def:ac-of-mc}. We prove Proposition \ref{prop-mc-to-ac} by indicating that for each state $s_i$ in $\M$, its corresponding node $n_i^+$ in $\mathcal{C}_{\M}$ and the weight function $w$ that agrees with $G$, $Pr_{\M,s_i}(\lozenge G)$ and $\mathcal{C}(n^+_i)[w]$ coincide.


\par \noindent Recall from Section \ref{sec:pmc} that for the state $s_i$, we denote the probability to reach the goal states $G$ by $p_{s_i}$. We show the correspondence for the following three cases: whether $s_i \in G$, whether $S_G$ is not reachable from $s$, and otherwise as characterized by equation (\ref{eq:equation-system}). 

\begin{itemize}
    \item For $s_i \in G$, we immediately have $p_{s_i} = 1$. For the corresponding node $n^+_i$, we have $C(n^+_i) = $ \textcolor{blue}{continue} as $op(n^+_i) = +$ and $n^+_i$ is a sum node by definition.
\end{itemize}
    
\end{proof}








\begin{proof}[Proof of Proposition \ref{prop-ac-to-mc}]
    
\end{proof}
